# Supplementary material for: Multi-sensor Joint Adaptive Birth Sampler for Labeled Random Finite Set Tracking
Source: arXiv:2109.04355 source file (2022-04-29)
Supplement: Supplementary file 1 [file appendix_sampling_distr.tex]

\section{Proof of Theorem~\ref{prop::cnd_likelihood}}\label{sec::appendix::sampling_distr}

% ------------------------ %
% Proof
% ------------------------ %
\begin{proof}

Since a known, bijective map $\theta' : \mathbb{B}_+ \rightarrow \mathbb{J}_0$, we can state that, if $\theta'(l_+) = J$, then the probability of label $l_+$ is proportional to the joint distribution of $J$ such that $p(J) \propto p(l_+)$.
By definition, the conditional distribution is proportional to the joint distribution by
\begin{equation*}
p(j^{(s)} | J^{-s}) = \frac{p(J)}{p(J^{-s})} \propto p(l_+).
\end{equation*}
Using Equation~(\ref{eq::orig_sampling_distr}) and, since all terms in the product $\left[1 - r_U\right]^{J}$ are not a function of $j^{(s)}$ except, $(1-r_U(z^{(s)}_{j^{(s)}})$, then we can roll those into the normalizing constant and reduce the expression to the final form,
\begin{equation*}
		p(j^{(s)} | J^{-s}) \propto \left(1 - r_U(z_{j^{(s)}})\right) \langle p_B, \psi^{J}_{Z}\rangle
\end{equation*}
\end{proof}
